# Supplementary material for: Fully Empirical Autotuned QR Factorization For Multicore Architectures
Source: arXiv:1102.5328 source file (2011-02-25)
Supplement: Supplementary file 1 [file appendix.tex]

\section{Detailed results}
\label{sec:details}

In this appendix, we present the extensive results that were collected
to produce Table%~\ref{table:val_conroe}.

\begin{table}[ht]
\caption{Performance of ES on the Intel Tigerton} % title of
\centering      % used for centering table 
\begin{tabular}{r r r r r}  % centered columns (4 columns) 
\hline\hline                        %inserts double horizontal lines 
N & ncore & Perf (Gflop/s) & NB & IB \\ [0.5ex] % inserts table 
%heading 
\hline                    % inserts single horizontal line 
2000	&4	&23.84	&156	&52\\
2000	&16	&69.71	&156	&52\\
6000	&4	&28.74	&300	&60\\
6000	&16	&99.27	&208	&52\\
\hline                    % inserts single horizontal line 
2700	&4	&25.93	&208	&52\\
2700	&16	&80.13	&180	&60\\
4200	&4	&27.8	&300	&60\\
4200	&16	&92.13	&156	&52\\
\hline                    % inserts single horizontal line 
2000	&7	&39	    &156	&52\\
2000	&10	&51.01	&156	&52\\
6000	&7	&49.31	&300	&60\\
6000	&10	&64.41	&208	&52\\
\hline                    % inserts single horizontal line 
2700	&7	&43.67	&208	&52\\
2700	&10	&57.67	&180	&60\\
4200	&7	&47.14	&300	&60\\
4200	&10	&61.97	&300	&60\\[1ex]
\hline                    % inserts single horizontal line 
% [1ex] adds vertical space 
\end{tabular}
\label{table:trigeton_ES}  % is used to refer this table in the text 
\end{table}

\begin{table}[ht] 
\caption{Performance of Heuristic~0 on the Intel Trigerton machine.} % title of Table
\centering      % used for centering table 
\begin{tabular}{r r r r r r r r } % centered columns (4 columns) 
\hline\hline                        %inserts double horizontal lines 
N & ncore& Y &PS &$\frac{PS}{ES}\%$& PSPAYG & $\frac{PSPAYG}{ES}\%$&$\frac{PSPAYG}{PS}\%$\\ [0.5ex]
%heading 
\hline                    % inserts single horizontal line 
2000	&	4	&	1	&	23.84	&	100	&	23.68	&	99.33	&	99.33	\\
2000	&	16	&	1	&	69.71	&	100	&	69.71	&	100	&	100	\\
6000	&	4	&	1	&	28.74	&	100	&	28.64	&	99.66	&	99.66	\\
6000	&	16	&	1	&	99.27	&	100	&	99.27	&	100	&	100	\\
\hline                    % inserts single horizontal line 
2700	&	4	&	1	&	23.69	&	91.36	&	25.03	&	96.52	&	105.65	\\
2700	&	16	&	1	&	77.86	&	97.17	&	77.86	&	97.17	&	100	\\
4200	&	4	&	1	&	27	&	97.09	&	27	&	97.09	&	100	\\
4200	&	16	&	1	&	92.13	&	100	&	92.13	&	100	&	100	\\
\hline                    % inserts single horizontal line 
2000	&	7	&	1	&	39	&	100	&	39	&	100	&	100	\\
2000	&	10	&	1	&	51.01	&	100	&	51.01	&	100	&	100	\\
6000	&	7	&	1	&	49.31	&	100	&	48.72	&	98.79	&	98.79	\\
6000	&	10	&	1	&	63.96	&	99.29	&	63.91	&	99.22	&	99.93	\\
\hline                    % inserts single horizontal line 
2700	&	7	&	1	&	39.63	&	90.75	&	39.63	&	90.75	&	100	\\
2700	&	10	&	1	&	54.83	&	95.07	&	54.83	&	95.07	&	100	\\
4200	&	7	&	1	&	44.46	&	94.3	&	44.46	&	94.3	&	100	\\
4200	&	10	&	1	&	57.46	&	92.72	&	57.46	&	92.72	&	100	\\[1ex]
\hline                    % inserts single horizontal line 
% [1ex] adds vertical space 
\end{tabular} 
\label{table:trigerton_H0}  % is used to refer this table in the text 
\end{table} 

\begin{table}[ht] 
\caption{Performance of Heuristic~1 on the Intel Trigerton machine} % title of Table 
\centering      % used for centering table 
\begin{tabular}{r r r r r r r r } % centered columns (4 columns) 
\hline\hline                        %inserts double horizontal lines 
N & ncore& Y &PS &$\frac{PS}{ES}\%$& PSPAYG & $\frac{PSPAYG}{ES}\%$&$\frac{PSPAYG}{PS}\%$\\ [0.5ex]
%heading 
\hline                    % inserts single horizontal line 
2000	&	4	&	0	&	21.73	&	91.12	&	21.73	&	91.12	&	100	\\
2000	&	16	&	0	&	68.19	&	97.81	&	68.19	&	97.81	&	100	\\
6000	&	4	&	0	&	27.15	&	94.46	&	27.15	&	94.46	&	100	\\
6000	&	16	&	0	&	87.21	&	87.85	&	87.21	&	87.85	&	100	\\
\hline                    % inserts single horizontal line 
2700	&	4	&	0	&	23.09	&	89.06	&	23.09	&	89.06	&	100	\\
2700	&	16	&	0	&	79.26	&	98.92	&	79.26	&	98.92	&	100	\\
4200	&	4	&	0	&	24.02	&	86.38	&	24.02	&	86.38	&	100	\\
4200	&	16	&	0	&	86.08	&	93.43	&	86.08	&	93.43	&	100	\\
\hline                    % inserts single horizontal line 
2000	&	7	&	0	&	36.03	&	92.39	&	36.03	&	92.39	&	100	\\
2000	&	10	&	0	&	48.75	&	95.57	&	48.75	&	95.57	&	100	\\
6000	&	7	&	0	&	45.22	&	91.7	&	45.22	&	91.7	&	100	\\
6000	&	10	&	0	&	55.99	&	86.93	&	55.99	&	86.93	&	100	\\
\hline                    % inserts single horizontal line 
2700	&	7	&	0	&	39.23	&	89.82	&	39.23	&	89.82	&	100	\\
2700	&	10	&	0	&	53.73	&	93.17	&	53.73	&	93.17	&	100	\\
4200	&	7	&	0	&	40.66	&	86.24	&	40.66	&	86.24	&	100	\\
4200	&	10	&	0	&	56.37	&	90.97	&	56.37	&	90.97	&	100	\\[1ex]
\hline                    % inserts single horizontal line 
% [1ex] adds vertical space 
\end{tabular} 
\label{table:tigerton_H1}  % is used to refer this table in the text 
\end{table} 

\begin{table}[ht] 
\caption{Performance of Heuristic~2 on the Intel Trigerton machine} % title of Table 
\centering      % used for centering table 
\begin{tabular}{r r r r r r r r } % centered columns (4 columns) 
\hline\hline                        %inserts double horizontal lines 
N & ncore& Y &PS &$\frac{PS}{ES}\%$& PSPAYG & \bf $\frac{PSPAYG}{ES}\%$&$\frac{PSPAYG}{PS}\%$\\ [0.5ex]
%heading 
\hline                    % inserts single horizontal line 
2000	&	4	&	1	&	23.84	&	100	&	23.68	&	99.33	&	99.33	\\
2000	&	16	&	1	&	69.71	&	100	&	69.71	&	100	&	100	\\
6000	&	4	&	1	&	28.74	&	100	&	28.74	&	100	&	100	\\
6000	&	16	&	1	&	99.27	&	100	&	99.27	&	100	&	100	\\
\hline                    % inserts single horizontal line 
2700	&	4	&	1	&	23.69	&	91.36	&	25.03	&	96.52	&	105.65	\\
2700	&	16	&	0	&	77.86	&	97.17	&	77.86	&	97.17	&	100	\\
4200	&	4	&	1	&	26.37	&	94.83	&	26.37	&	94.83	&	100	\\
4200	&	16	&	1	&	92.13	&	100	&	92.13	&	100	&	100	\\
\hline                    % inserts single horizontal line 
2000	&	7	&	1	&	39	&	100	&	39	&	100	&	100	\\
2000	&	10	&	1	&	51.01	&	100	&	51.01	&	100	&	100	\\
6000	&	7	&	1	&	49.31	&	100	&	49.31	&	100	&	100	\\
6000	&	10	&	1	&	63.96	&	99.29	&	63.96	&	99.29	&	100	\\
\hline                    % inserts single horizontal line 
2700	&	7	&	1	&	39.63	&	90.75	&	39.63	&	90.75	&	100	\\
2700	&	10	&	0	&	54.83	&	95.07	&	54.83	&	95.07	&	100	\\
4200	&	7	&	1	&	44.15	&	93.64	&	44.15	&	93.64	&	100	\\
4200	&	10	&	1	&	60.73	&	98.01	&	60.73	&	98.01	&	100	\\[1ex]
\hline                    % inserts single horizontal line 
\end{tabular} 
\label{table:tigerton_H2}  % is used to refer this table in the text 
\end{table}

\begin{table}[ht]
\caption{Performance of ES on the Intel Nehalem} % title of
\centering      % used for centering table 
\begin{tabular}{r r r r r}  % centered columns (4 columns) 
\hline\hline                        %inserts double horizontal lines 
N & ncore & Perf (Gflop/s) & NB & IB \\ [0.5ex] % inserts table 
%heading 
\hline                    % inserts single horizontal line 
2000	&	4	&	34.73	&	168	&	56	\\
2000	&	8	&	62.69	&	168	&	56	\\
6000	&	4	&	39.24	&	240	&	60	\\
6000	&	8	&	73.07	&	240	&	60	\\
\hline                    % inserts single horizontal line 
2700	&	4	&	35.24	&	240	&	60	\\
2700	&	8	&	63.28	&	168	&	56	\\
4200	&	4	&	37.14	&	240	&	60	\\
4200	&	8	&	70.03	&	168	&	56	\\
\hline                    % inserts single horizontal line 
2000	&	2	&	18.67	&	504	&	72	\\
2000	&	7	&	56.46	&	168	&	56	\\
6000	&	2	&	21.68	&	504	&	72	\\
6000	&	7	&	66	&	240	&	60	\\
\hline                    % inserts single horizontal line 
2700	&	2	&	19.79	&	480	&	80	\\
2700	&	7	&	55.53	&	240	&	60	\\
4200	&	2	&	21.2	&	480	&	80	\\
4200	&	7	&	62.54	&	168	&	56	\\[1ex]
\hline                    % inserts single horizontal line 
% [1ex] adds vertical space 
\end{tabular}
\label{table:Nehalem_ES}  % is used to refer this table in the text 
\end{table}

\begin{table}[ht] 
\caption{Performance of Heuristic~0 on the Intel Nehalem machine.} % title of Table
\centering      % used for centering table 
\begin{tabular}{r r r r r r r r } % centered columns (4 columns) 
\hline\hline                        %inserts double horizontal lines 
N & ncore& Y &PS &$\frac{PS}{ES}\%$& PSPAYG & $\frac{PSPAYG}{ES}\%$&$\frac{PSPAYG}{PS}\%$\\ [0.5ex]
%heading 
\hline                    % inserts single horizontal line 
2000	&	4	&	1	&	34.73	&	100	&	34.73	&	100	&	100	\\
2000	&	8	&	1	&	62.48	&	99.67	&	62.48	&	99.67	&	100	\\
6000	&	4	&	1	&	39.24	&	100	&	39.24	&	100	&	100	\\
6000	&	8	&	1	&	73.07	&	100	&	73.07	&	100	&	100	\\
\hline     %inserts single line 
2700	&	4	&	1	&	34.05	&	96.63	&	34.05	&	96.63	&	100	\\
2700	&	8	&	1	&	61.47	&	97.13	&	61.47	&	97.13	&	100	\\
4200	&	4	&	1	&	37.14	&	100	&	37.14	&	100	&	100	\\
4200	&	8	&	1	&	70.03	&	100	&	70.03	&	100	&	100	\\
\hline     %inserts single line 
2000	&	2	&	1	&	18.46	&	98.88	&	18.52	&	99.2	&	100.32	\\
2000	&	7	&	1	&	55.85	&	98.92	&	55.85	&	98.92	&	100	\\
6000	&	2	&	1	&	21.68	&	100	&	21.68	&	100	&	100	\\
6000	&	7	&	1	&	66	&	100	&	66	&	100	&	100	\\
\hline     %inserts single line 
2700	&	2	&	1	&	18.02	&	91.04	&	18.9	&	95.51	&	104.92	\\
2700	&	7	&	1	&	54.77	&	98.62	&	54.77	&	98.62	&	100	\\
4200	&	2	&	1	&	20.5	&	96.7	&	20.5	&	96.7	&	100	\\
4200	&	7	&	1	&	62.54	&	100	&	62.54	&	100	&	100	\\[1ex]
% [1ex] adds vertical space 
\hline     %inserts single line 
\end{tabular} 
\label{table:Nehalem_H0}  % is used to refer this table in the text 
\end{table} 

\begin{table}[ht] 
\caption{Performance of Heuristic~1 on the Intel Nehalem machine} % title of Table 
\centering      % used for centering table 
\begin{tabular}{r r r r r r r r } % centered columns (4 columns) 
\hline\hline                        %inserts double horizontal lines 
N & ncore& Y &PS &$\frac{PS}{ES}\%$& PSPAYG & $\frac{PSPAYG}{ES}\%$&$\frac{PSPAYG}{PS}\%$\\ [0.5ex]
%heading 
\hline                    % inserts single horizontal line 
2000	&	4	&	1	&	34.73	&	100	&	34.73	&	100	&	100	\\
2000	&	8	&	1	&	62.48	&	99.67	&	62.48	&	99.67	&	100	\\
6000	&	4	&	1	&	39.24	&	100	&	39.24	&	100	&	100	\\
6000	&	8	&	1	&	73.07	&	100	&	73.07	&	100	&	100	\\
\hline     %inserts single line 
2700	&	4	&	1	&	34.05	&	96.63	&	34.05	&	96.63	&	100	\\
2700	&	8	&	1	&	61.47	&	97.13	&	61.47	&	97.13	&	100	\\
4200	&	4	&	1	&	37.14	&	100	&	37.14	&	100	&	100	\\
4200	&	8	&	1	&	70.03	&	100	&	70.03	&	100	&	100	\\
\hline     %inserts single line 
2000	&	2	&	1	&	18.46	&	98.88	&	18.52	&	99.2	&	100.32	\\
2000	&	7	&	1	&	55.85	&	98.92	&	55.85	&	98.92	&	100	\\
6000	&	2	&	1	&	21.68	&	100	&	21.68	&	100	&	100	\\
6000	&	7	&	1	&	66	&	100	&	66	&	100	&	100	\\
\hline     %inserts single line 
2700	&	2	&	1	&	18.02	&	91.04	&	18.9	&	95.51	&	104.92	\\
2700	&	7	&	1	&	54.77	&	98.62	&	54.77	&	98.62	&	100	\\
4200	&	2	&	1	&	20.5	&	96.7	&	20.5	&	96.7	&	100	\\
4200	&	7	&	1	&	62.54	&	100	&	62.54	&	100	&	100	\\[1ex]
% [1ex] adds vertical space 
\hline     %inserts single line 
\end{tabular} 
\label{table:Nehalem_H1}  % is used to refer this table in the text 
\end{table} 

\begin{table}[ht] 
\caption{Performance of Heuristic~2 on the Intel Nehalem machine} % title of Table 
\centering      % used for centering table 
\begin{tabular}{r r r r r r r r } % centered columns (4 columns) 
\hline\hline                        %inserts double horizontal lines 
N & ncore& Y &PS &$\frac{PS}{ES}\%$& PSPAYG & \bf $\frac{PSPAYG}{ES}\%$&$\frac{PSPAYG}{PS}\%$\\ [0.5ex]
%heading 
\hline                    % inserts single horizontal line 
2000	&	4	&	1	&	34.73	&	100	&	34.73	&	100	&	100	\\
2000	&	8	&	1	&	62.48	&	99.67	&	62.48	&	99.67	&	100	\\
6000	&	4	&	1	&	39.24	&	100	&	39.24	&	100	&	100	\\
6000	&	8	&	1	&	73.07	&	100	&	73.07	&	100	&	100	\\
\hline                    % inserts single horizontal line 
2700	&	4	&	1	&	34.05	&	96.63	&	34.05	&	96.63	&	100	\\
2700	&	8	&	1	&	61.47	&	97.13	&	61.47	&	97.13	&	100	\\
4200	&	4	&	1	&	37.14	&	100	&	37.14	&	100	&	100	\\
4200	&	8	&	1	&	70.03	&	100	&	70.03	&	100	&	100	\\
\hline                    % inserts single horizontal line 
2000	&	2	&	1	&	18.46	&	98.88	&	18.52	&	99.2	&	100.32	\\
2000	&	7	&	1	&	55.85	&	98.92	&	55.85	&	98.92	&	100	\\
6000	&	2	&	1	&	21.68	&	100	&	21.68	&	100	&	100	\\
6000	&	7	&	1	&	66	&	100	&	66	&	100	&	100	\\
\hline                    % inserts single horizontal line 
2700	&	2	&	1	&	18.02	&	91.04	&	18.9	&	95.51	&	104.92	\\
2700	&	7	&	1	&	54.77	&	98.62	&	54.77	&	98.62	&	100	\\
4200	&	2	&	1	&	20.5	&	96.7	&	20.5	&	96.7	&	100	\\
4200	&	7	&	1	&	62.54	&	100	&	62.54	&	100	&	100	\\[1ex]
\hline     %inserts single line 
\end{tabular} 
\label{table:Nehalem_H2}  % is used to refer this table in the text 
\end{table}

\begin{table}[ht]
\caption{Performance of ES on the Intel Clovertown} % title of
\centering      % used for centering table 
\begin{tabular}{r r r r r}  % centered columns (4 columns) 
\hline\hline                        %inserts double horizontal lines 
N & ncore & Perf (Gflop/s) & NB & IB \\ [0.5ex] % inserts table 
%heading 
\hline                    % inserts single horizontal line 
2000	&	4	&	26.29	&	156	&	52	\\
2000	&	8	&	45.43	&	156	&	52	\\
6000	&	4	&	31.23	&	300	&	60	\\
6000	&	8	&	51.84	&	180	&	60	\\
\hline                    % inserts single horizontal line 
2700	&	4	&	28.31	&	300	&	60	\\
2700	&	8	&	48.88	&	180	&	60	\\
4200	&	4	&	30.38	&	300	&	60	\\
4200	&	8	&	51.73	&	156	&	52	\\
\hline                    % inserts single horizontal line 
2000	&	3	&	20.76	&	300	&	60	\\
2000	&	7	&	39.96	&	156	&	52	\\
6000	&	3	&	23.38	&	360	&	60	\\
6000	&	7	&	44.53	&	192	&	64	\\
\hline                    % inserts single horizontal line 
2700	&	3	&	21.67	&	300	&	60	\\
2700	&	7	&	42.58	&	180	&	60	\\
4200	&	3	&	22.74	&	300	&	60	\\
4200	&	7	&	43.81	&	156	&	52	\\[1ex]
\hline                    % inserts single horizontal line 
% [1ex] adds vertical space 
\end{tabular}
\label{table:Clovertown_ES}  % is used to refer this table in the text 
\end{table}

\begin{table}[ht] 
\caption{Performance of Heuristic~0 on the Intel Clovertown machine.} % title of Table
\centering      % used for centering table 
\begin{tabular}{r r r r r r r r } % centered columns (4 columns) 
\hline\hline                        %inserts double horizontal lines 
N & ncore& Y &PS &$\frac{PS}{ES}\%$& PSPAYG & $\frac{PSPAYG}{ES}\%$&$\frac{PSPAYG}{PS}\%$\\ [0.5ex]
%heading 
\hline                    % inserts single horizontal line 
2000	&	4	&	1	&	26.29	&	100	&	26.29	&	100	&	100	\\
2000	&	8	&	1	&	45.43	&	100	&	45.43	&	100	&	100	\\
6000	&	4	&	1	&	31.23	&	100	&	31.23	&	100	&	100	\\
6000	&	8	&	1	&	51.82	&	99.95	&	51.82	&	99.95	&	100	\\
\hline                    % inserts single horizontal line 
2700	&	4	&	1	&	26	&	91.84	&	26	&	91.84	&	100	\\
2700	&	8	&	1	&	46.74	&	95.62	&	46.74	&	95.62	&	100	\\
4200	&	4	&	1	&	28.61	&	94.19	&	28.61	&	94.19	&	100	\\
4200	&	8	&	1	&	51.62	&	99.78	&	51.62	&	99.78	&	100	\\
\hline                    % inserts single horizontal line 
2000	&	3	&	1	&	20.76	&	100	&	20.76	&	100	&	100	\\
2000	&	7	&	1	&	39.96	&	100	&	39.96	&	100	&	100	\\
6000	&	3	&	1	&	23.38	&	100	&	22.48	&	96.16	&	96.16	\\
6000	&	7	&	1	&	44.53	&	100	&	44.53	&	100	&	100	\\
\hline                    % inserts single horizontal line 
2700	&	3	&	1	&	21.67	&	100	&	21.67	&	100	&	100	\\
2700	&	7	&	1	&	41.28	&	96.97	&	41.28	&	96.97	&	100	\\
4200	&	3	&	1	&	22.66	&	99.67	&	22.66	&	99.67	&	100	\\
4200	&	7	&	1	&	43.52	&	99.35	&	43.52	&	99.35	&	100	\\[1ex]
\hline                    % inserts single horizontal line 
% [1ex] adds vertical space 
\hline     %inserts single line 
\end{tabular} 
\label{table:Clovertown_H0}  % is used to refer this table in the text 
\end{table} 

\begin{table}[ht] 
\caption{Performance of Heuristic~1 on the Intel Clovertown machine} % title of Table 
\centering      % used for centering table 
\begin{tabular}{r r r r r r r r } % centered columns (4 columns) 
\hline\hline                        %inserts double horizontal lines 
N & ncore& Y &PS &$\frac{PS}{ES}\%$& PSPAYG & $\frac{PSPAYG}{ES}\%$&$\frac{PSPAYG}{PS}\%$\\ [0.5ex]
%heading 
\hline                    % inserts single horizontal line 
2000	&	4	&	0	&	24.22	&	92.13	&	24.22	&	92.13	&	100	\\
2000	&	8	&	0	&	43.58	&	95.92	&	43.58	&	95.92	&	100	\\
6000	&	4	&	0	&	28.06	&	89.85	&	28.06	&	89.85	&	100	\\
6000	&	8	&	0	&	47.77	&	92.15	&	47.77	&	92.15	&	100	\\
\hline     %inserts single line 
2700	&	4	&	0	&	25.51	&	90.14	&	25.51	&	90.14	&	100	\\
2700	&	8	&	0	&	46.02	&	94.16	&	46.02	&	94.16	&	100	\\
4200	&	4	&	0	&	25.09	&	82.59	&	25.09	&	82.59	&	100	\\
4200	&	8	&	0	&	47.58	&	91.98	&	47.58	&	91.98	&	100	\\
\hline     %inserts single line 
2000	&	3	&	0	&	17.65	&	85.03	&	17.65	&	85.03	&	100	\\
2000	&	7	&	0	&	38.67	&	96.79	&	38.67	&	96.79	&	100	\\
6000	&	3	&	0	&	21.97	&	93.97	&	21.97	&	93.97	&	100	\\
6000	&	7	&	0	&	42.26	&	94.9	&	42.26	&	94.9	&	100	\\
\hline     %inserts single line 
2700	&	3	&	0	&	18.77	&	86.62	&	18.77	&	86.62	&	100	\\
2700	&	7	&	0	&	41.52	&	97.51	&	41.52	&	97.51	&	100	\\
4200	&	3	&	0	&	20.4	&	89.72	&	20.4	&	89.72	&	100	\\
4200	&	7	&	0	&	42.01	&	95.9	&	42.01	&	95.9	&	100	\\[1ex]
% [1ex] adds vertical space 
\hline     %inserts single line 
\end{tabular} 
\label{table:Clovertown_H1}  % is used to refer this table in the text 
\end{table} 

\begin{table}[ht] 
\caption{Performance of Heuristic~2 on the Intel Clovertown machine} % title of Table 
\centering      % used for centering table 
\begin{tabular}{r r r r r r r r } % centered columns (4 columns) 
\hline\hline                        %inserts double horizontal lines 
N & ncore& Y &PS &$\frac{PS}{ES}\%$& PSPAYG & \bf $\frac{PSPAYG}{ES}\%$&$\frac{PSPAYG}{PS}\%$\\ [0.5ex]
%heading 
\hline                    % inserts single horizontal line 
2000	&	4	&	1	&	26.29	&	100	&	26.29	&	100	&	100	\\
2000	&	8	&	1	&	45.43	&	100	&	45.43	&	100	&	100	\\
6000	&	4	&	1	&	31.23	&	100	&	31.23	&	100	&	100	\\
6000	&	8	&	0	&	51.63	&	99.59	&	51.63	&	99.59	&	100	\\
\hline     %inserts single line 
2700	&	4	&	1	&	26	&	91.84	&	26	&	91.84	&	100	\\
2700	&	8	&	0	&	46.74	&	95.62	&	46.74	&	95.62	&	100	\\
4200	&	4	&	1	&	28.61	&	94.19	&	28.61	&	94.19	&	100	\\
4200	&	8	&	1	&	51.73	&	100	&	51.73	&	100	&	100	\\
\hline     %inserts single line 
2000	&	3	&	1	&	20.76	&	100	&	20.76	&	100	&	100	\\
2000	&	7	&	1	&	39.96	&	100	&	39.96	&	100	&	100	\\
6000	&	3	&	1	&	23.38	&	100	&	22.48	&	96.16	&	96.16	\\
6000	&	7	&	0	&	43.59	&	97.89	&	43.59	&	97.89	&	100	\\
\hline     %inserts single line 
2700	&	3	&	1	&	21.67	&	100	&	21.67	&	100	&	100	\\
2700	&	7	&	0	&	41.28	&	96.97	&	41.28	&	96.97	&	100	\\
4200	&	3	&	1	&	22.66	&	99.67	&	22.66	&	99.67	&	100	\\
4200	&	7	&	1	&	43.81	&	100	&	43.81	&	100	&	100	\\[1ex]
\hline     %inserts single line 
\end{tabular} 
\label{table:Clovertown_H2}  % is used to refer this table in the text 
\end{table}

\begin{table}[ht]
\caption{Performance of ES on the Intel Yorkfield} % title of
\centering      % used for centering table 
\begin{tabular}{r r r r r}  % centered columns (4 columns) 
\hline\hline                        %inserts double horizontal lines 
N & ncore & Perf (Gflop/s) & NB & IB \\ [0.5ex] % inserts table 
%heading 
\hline                    % inserts single horizontal line 
2000	&	2	&	14.67	&	300	&	60	\\
2000	&	4	&	26.2	&	156	&	52	\\
6000	&	2	&	15.93	&	364	&	52	\\
6000	&	4	&	29.32	&	240	&	60	\\
\hline                    % inserts single horizontal line 
2700	&	2	&	15.02	&	300	&	60	\\
2700	&	4	&	27.45	&	180	&	60	\\
4200	&	2	&	15.74	&	364	&	52	\\
4200	&	4	&	27.99	&	156	&	52	\\
\hline                    % inserts single horizontal line 
2000	&	3	&	20.23	&	156	&	52	\\
6000	&	3	&	22.4	&	300	&	60	\\
\hline                    % inserts single horizontal line 
2700	&	3	&	21.56	&	300	&	60	\\
4200	&	3	&	21.98	&	300	&	60	\\[1ex]
\hline                    % inserts single horizontal line 
% [1ex] adds vertical space 
\end{tabular}
\label{table:Yorkfield_ES}  % is used to refer this table in the text 
\end{table}

\begin{table}[ht] 
\caption{Performance of Heuristic~0 on the Intel Yorkfield machine.} % title of Table
\centering      % used for centering table 
\begin{tabular}{r r r r r r r r } % centered columns (4 columns) 
\hline\hline                        %inserts double horizontal lines 
N & ncore& Y &PS &$\frac{PS}{ES}\%$& PSPAYG & $\frac{PSPAYG}{ES}\%$&$\frac{PSPAYG}{PS}\%$\\ [0.5ex]
%heading 
\hline                    % inserts single horizontal line 
2000	&	2	&	1	&	14.67	&	100	&	14.67	&	100	&	100	\\
2000	&	4	&	1	&	26.2	&	100	&	26.2	&	100	&	100	\\
6000	&	2	&	1	&	15.93	&	100	&	15.93	&	100	&	100	\\
6000	&	4	&	1	&	29.32	&	100	&	29.32	&	100	&	100	\\
\hline     %inserts single line 
2700	&	2	&	1	&	15.02	&	100	&	15.02	&	100	&	100	\\
2700	&	4	&	1	&	25.86	&	94.21	&	25.86	&	94.21	&	100	\\
4200	&	2	&	1	&	15.74	&	100	&	15.74	&	100	&	100	\\
4200	&	4	&	1	&	27.86	&	99.54	&	27.86	&	99.54	&	100	\\
\hline     %inserts single line 
2000	&	3	&	1	&	20.16	&	99.65	&	20.16	&	99.65	&	100	\\
6000	&	3	&	1	&	21.54	&	96.15	&	21.54	&	96.15	&	100	\\
\hline     %inserts single line 
2700	&	3	&	1	&	21.56	&	100	&	21.56	&	100	&	100	\\
4200	&	3	&	1	&	21.22	&	96.53	&	21.22	&	96.53	&	100	\\[1ex]
% [1ex] adds vertical space 
\hline     %inserts single line 
\end{tabular} 
\label{table:Yorkfield_H0}  % is used to refer this table in the text 
\end{table} 

\begin{table}[ht] 
\caption{Performance of Heuristic~1 on the Intel Yorkfield machine} % title of Table 
\centering      % used for centering table 
\begin{tabular}{r r r r r r r r } % centered columns (4 columns) 
\hline\hline                        %inserts double horizontal lines 
N & ncore& Y &PS &$\frac{PS}{ES}\%$& PSPAYG & $\frac{PSPAYG}{ES}\%$&$\frac{PSPAYG}{PS}\%$\\ [0.5ex]
\hline                    % inserts single horizontal line 
2000	&	2	&		0	&	12.85	&	87.61	&	12.72	&	86.68	&	98.93	\\
2000	&	4	&		0	&	24.28	&	92.69	&	24.28	&	92.69	&	100	\\
6000	&	2	&		0	&	15.23	&	95.59	&	15.23	&	95.59	&	100	\\
6000	&	4	&		0	&	27.41	&	93.49	&	27.41	&	93.49	&	100	\\
\hline                    % inserts single horizontal line 
2700	&	2	&		0	&	13.25	&	88.22	&	13.58	&	90.4	&	102.47	\\
2700	&	4	&		0	&	25.39	&	92.48	&	25.39	&	92.48	&	100	\\
4200	&	2	&		0	&	13.83	&	87.82	&	13.83	&	87.82	&	100	\\
4200	&	4	&		0	&	27.22	&	97.26	&	27.22	&	97.26	&	100	\\
\hline                    % inserts single horizontal line 
2000	&	3	&		0	&	18.64	&	92.13	&	18.48	&	91.34	&	99.14	\\
6000	&	3	&		0	&	21.51	&	96.02	&	21.51	&	96.02	&	100	\\
\hline                    % inserts single horizontal line 
2700	&	3	&		0	&	19.17	&	88.94	&	19.24	&	89.25	&	100.36	\\
4200	&	3	&		0	&	18.93	&	86.11	&	18.93	&	86.11	&	100	\\[1ex]
%heading 
% [1ex] adds vertical space 
\hline     %inserts single line 
\end{tabular} 
\label{table:Yorkfield_H1}  % is used to refer this table in the text 
\end{table} 

\begin{table}[ht] 
\caption{Performance of Heuristic~2 on the Intel Yorkfield machine} % title of Table 
\centering      % used for centering table 
\begin{tabular}{r r r r r r r r } % centered columns (4 columns) 
\hline\hline                        %inserts double horizontal lines 
N & ncore& Y &PS &$\frac{PS}{ES}\%$& PSPAYG & $\frac{PSPAYG}{ES}\%$&$\frac{PSPAYG}{PS}\%$\\ [0.5ex]
\hline                    % inserts single horizontal line 
2000	&	2	&	1	&	14.67	&	100	&	14.67	&	100	&	100	\\
2000	&	4	&	1	&	26.2	&	100	&	26.2	&	100	&	100	\\
6000	&	2	&	1	&	15.93	&	100	&	15.93	&	100	&	100	\\
6000	&	4	&	0	&	28.96	&	98.78	&	28.96	&	98.78	&	100	\\
\hline                    % inserts single horizontal line 
2700	&	2	&	1	&	15.02	&	100	&	15.02	&	100	&	100	\\
2700	&	4	&	0	&	25.86	&	94.21	&	25.86	&	94.21	&	100	\\
4200	&	2	&	1	&	15.74	&	100	&	15.74	&	100	&	100	\\
4200	&	4	&	1	&	27.5	&	98.25	&	27.5	&	98.25	&	100	\\
\hline                    % inserts single horizontal line 
2000	&	3	&	1	&	20.16	&	99.65	&	20.16	&	99.65	&	100	\\
6000	&	3	&	1	&	21.54	&	96.15	&	21.54	&	96.15	&	100	\\
\hline                    % inserts single horizontal line 
2700	&	3	&	1	&	21.56	&	100	&	21.56	&	100	&	100	\\
4200	&	3	&	1	&	21.22	&	96.53	&	21.22	&	96.53	&	100	\\
%heading 
% [1ex] adds vertical space 
\hline     %inserts single line 
\end{tabular} 
\label{table:Yorkfield_H2}  % is used to refer this table in the text 
\end{table}
