# Supplementary material for: Fully Empirical Autotuned QR Factorization For Multicore Architectures
Source: arXiv:1102.5328 source file (2011-02-25)
Supplement: Supplementary file 2 [file appendix2.tex]

\section{Detailed results}
\label{sec:details}

In this appendix, we present the extensive results that were collected
to produce Table%~\ref{table:val_conroe}.

\begin{table}[ht]
\caption{Performance of ES on the Intel Conroe} % title of
\centering      % used for centering table 
\begin{tabular}{r r r r r}  % centered columns (4 columns) 
\hline\hline                        %inserts double horizontal lines 
N & ncore & Perf (Gflop/s) & NB & IB \\ [0.5ex] % inserts table 
%heading 
\hline                    % inserts single horizontal line 
2000    &   1   &   7.05    &   420 &   60  \\
2000    &   2   &   12.54   &   420 &   60  \\
6000    &   1   &   7.5 &   420 &   60  \\
6000    &   2   &   13.84   &   504 &   72  \\
\hline                    % inserts single horizontal line 
2700    &   1   &   7.22    &   480 &   60  \\
2700    &   2   &   13.14   &   280 &   56  \\
4200    &   1   &   7.45    &   420 &   60  \\
4200    &   2   &   13.64   &   392 &   56  \\[1ex]
\hline                    % inserts single horizontal line 
% [1ex] adds vertical space 
\end{tabular}
\label{table:Conroe_ES}  % is used to refer this table in the text 
\end{table}

\begin{table}[ht]
\caption{Performance of Heuristic~0 on the Intel Conroe machine.} % title of Table
\centering      % used for centering table 
\begin{tabular}{r r r r r r r r } % centered columns (4 columns) 
\hline\hline                        %inserts double horizontal lines 
N & ncore& Y &PS &$\frac{PS}{ES}\%$& PSPAYG & $\frac{PSPAYG}{ES}\%$&$\frac{PSPAYG}{PS}\%$\\ [0.5ex]
%heading 
\hline                    % inserts single horizontal line 
2000    &   1   &   1   &   7.05    &   100 &   7.05    &   100 &   100 \\
2000    &   2   &   1   &   12.54   &   100 &   12.54   &   100 &   100 \\
6000    &   1   &   1   &   7.5 &   100 &   7.5 &   100 &   100 \\
6000    &   2   &   1   &   13.84   &   100 &   13.84   &   100 &   100 \\
\hline     %inserts single line 
2700    &   1   &   1   &   7.2 &   99.76   &   7.2 &   99.76   &   100 \\
2700    &   2   &   1   &   12.83   &   97.59   &   12.83   &   97.59   &   100 \\
4200    &   1   &   1   &   7.45    &   100 &   7.45    &   100 &   100 \\
4200    &   2   &   1   &   13.64   &   100 &   13.64   &   100 &   100 \\[1ex]
\hline                    % inserts single horizontal line 
\end{tabular}
\label{table:Conroe_H0}  % is used to refer this table in the text 
\end{table}

\begin{table}[ht]
\caption{Performance of Heuristic~1 on the Intel Conroe machine.} % title of Table
\centering      % used for centering table 
\begin{tabular}{r r r r r r r r } % centered columns (4 columns) 
\hline\hline                        %inserts double horizontal lines 
N & ncore& Y &PS &$\frac{PS}{ES}\%$& PSPAYG & $\frac{PSPAYG}{ES}\%$&$\frac{PSPAYG}{PS}\%$\\ [0.5ex]
%heading 
\hline     %inserts single line 
2000    &   1   &   0   &   6.57    &   93.24   &   6.57    &   93.24   &   100 \\
2000    &   2   &   0   &   11.8    &   94.11   &   11.8    &   94.11   &   100 \\
6000    &   1   &   0   &   7.32    &   97.57   &   7.32    &   97.57   &   100 \\
6000    &   2   &   0   &   13.73   &   99.19   &   13.73   &   99.19   &   100 \\
\hline                    % inserts single horizontal line 
2700    &   1   &   0   &   6.75    &   93.51   &   6.75    &   93.51   &   100 \\
2700    &   2   &   0   &   12.86   &   97.83   &   12.86   &   97.83   &   100 \\
4200    &   1   &   0   &   7.08    &   95.11   &   7.08    &   95.11   &   100 \\
4200    &   2   &   0   &   12.51   &   91.66   &   12.51   &   91.66   &   100 \\[1ex]
\hline                    % inserts single horizontal line 
\end{tabular}
\label{table:Conroe_H1}  % is used to refer this table in the text 
\end{table}

\begin{table}[ht]
\caption{Performance of Heuristic~2 on the Intel Conroe machine.} % title of Table
\centering      % used for centering table 
\begin{tabular}{r r r r r r r r } % centered columns (4 columns) 
\hline\hline                        %inserts double horizontal lines 
N & ncore& Y &PS &$\frac{PS}{ES}\%$& PSPAYG & $\frac{PSPAYG}{ES}\%$&$\frac{PSPAYG}{PS}\%$\\ [0.5ex]
%heading 
\hline                    % inserts single horizontal line 
2000    &   1   &   1   &   7.05    &   100 &   7.05    &   100 &   100 \\
2000    &   2   &   1   &   12.54   &   100 &   12.54   &   100 &   100 \\
6000    &   1   &   1   &   7.5 &   100 &   7.5 &   100 &   100 \\
6000    &   2   &   0   &   13.7    &   99  &   13.7    &   99  &   100 \\
\hline                    % inserts single horizontal line 
2700    &   1   &   1   &   7.2 &   99.76   &   7.2 &   99.76   &   100 \\
2700    &   2   &   1   &   12.83   &   97.59   &   12.83   &   97.59   &   100 \\
4200    &   1   &   1   &   7.45    &   100 &   7.45    &   100 &   100 \\
4200    &   2   &   1   &   13.64   &   100 &   13.64   &   100 &   100 \\[1ex]
\hline                    % inserts single horizontal line 
\end{tabular}
\label{table:Conroe_H2}  % is used to refer this table in the text 
\end{table}

\begin{table}[ht]
\caption{Performance of ES on the IBM Power6} % title of
\centering      % used for centering table 
\begin{tabular}{r r r r r}  % centered columns (4 columns) 
\hline\hline                        %inserts double horizontal lines 
N & ncore & Perf (Gflop/s) & NB & IB \\ [0.5ex] % inserts table 
%heading 
\hline                    % inserts single horizontal line 
2000	&	8	&	55.97	&	168	&	28	\\
2000	&	32	&	85.14	&	96	&	32	\\
6000	&	8	&	81.67	&	504	&	56	\\
6000	&	32	&	255.83	&	168	&	28	\\
1000	&	1	&	9.23	&	300	&	60	\\
4000	&	1	&	11.44	&	108	&	36	\\
6000	&	1	&	11.72	&	480	&	60	\\
8000	&	1	&	12.05	&	128	&	32	\\
1000	&	2	&	14.85	&	168	&	28	\\
4000	&	2	&	21.83	&	96	&	32	\\
6000	&	2	&	22.99	&	300	&	60	\\
8000	&	2	&	23.4	&	168	&	28	\\
8000	&	8	&	85.35	&	180	&	36	\\
8000	&	32	&	264.36	&	108	&	36	\\
8000	&	8	&	85.35	&	300	&	60	\\
8000	&	32	&	264.36	&	168	&	28	\\[1ex]
\hline                    % inserts single horizontal line 
% [1ex] adds vertical space 
\end{tabular}
\label{table:Power6_ES}  % is used to refer this table in the text 
\end{table}

\begin{table}[ht]
\caption{Performance of Heuristic~0 on the IBM Power6 machine.} % title of Table
\centering      % used for centering table 
\begin{tabular}{r r r r r r r r } % centered columns (4 columns) 
\hline\hline                        %inserts double horizontal lines 
N & ncore& Y &PS &$\frac{PS}{ES}\%$& PSPAYG & $\frac{PSPAYG}{ES}\%$&$\frac{PSPAYG}{PS}\%$\\ [0.5ex]
%heading 
\hline                    % inserts single horizontal line 
2000	&	8	&	1	&	55.97	&	100	&	55.97	&	100	&	100	\\
2000	&	32	&	1	&	85.14	&	100	&	85.14	&	100	&	100	\\
6000	&	8	&	1	&	81.67	&	100	&	81.67	&	100	&	100	\\
6000	&	32	&	1	&	255.83	&	100	&	255.83	&	100	&	100	\\
1000	&	1	&	1	&	9.23	&	100	&	9.23	&	100	&	100	\\
4000	&	1	&	1	&	11.44	&	100	&	11.44	&	100	&	100	\\
6000	&	1	&	1	&	11.72	&	100	&	11.72	&	100	&	100	\\
8000	&	1	&	1	&	12.05	&	100	&	12.05	&	100	&	100	\\
1000	&	2	&	1	&	14.85	&	100	&	14.85	&	100	&	100	\\
4000	&	2	&	1	&	21.83	&	100	&	21.83	&	100	&	100	\\
6000	&	2	&	1	&	22.99	&	100	&	22.99	&	100	&	100	\\
8000	&	2	&	1	&	23.4	&	100	&	23.4	&	100	&	100	\\
8000	&	8	&	1	&	85.35	&	100	&	85.35	&	100	&	100	\\
8000	&	32	&	1	&	264.36	&	100	&	264.36	&	100	&	100	\\
8000	&	8	&	1	&	85.35	&	100	&	85.35	&	100	&	100	\\
8000	&	32	&	1	&	264.36	&	100	&	264.36	&	100	&	100	\\[1ex]
\hline                    % inserts single horizontal line 
\end{tabular}
\label{table:Power6_H0}  % is used to refer this table in the text 
\end{table}

\begin{table}[ht]
\caption{Performance of Heuristic~1 on the IBM Power6 machine.} % title of Table
\centering      % used for centering table 
\begin{tabular}{r r r r r r r r } % centered columns (4 columns) 
\hline\hline                        %inserts double horizontal lines 
N & ncore& Y &PS &$\frac{PS}{ES}\%$& PSPAYG & $\frac{PSPAYG}{ES}\%$&$\frac{PSPAYG}{PS}\%$\\ [0.5ex]
%heading 
\hline     %inserts single line 
2000	&	8	&	1	&	55.97	&	100	&	55.97	&	100	&	100	\\
2000	&	32	&	1	&	85.14	&	100	&	85.14	&	100	&	100	\\
6000	&	8	&	1	&	81.67	&	100	&	81.67	&	100	&	100	\\
6000	&	32	&	1	&	255.83	&	100	&	255.83	&	100	&	100	\\
1000	&	1	&	1	&	9.23	&	100	&	9.23	&	100	&	100	\\
4000	&	1	&	1	&	11.44	&	100	&	11.44	&	100	&	100	\\
6000	&	1	&	1	&	11.72	&	100	&	11.72	&	100	&	100	\\
8000	&	1	&	1	&	12.05	&	100	&	12.05	&	100	&	100	\\
1000	&	2	&	1	&	14.85	&	100	&	14.85	&	100	&	100	\\
4000	&	2	&	1	&	21.83	&	100	&	21.83	&	100	&	100	\\
6000	&	2	&	1	&	22.99	&	100	&	22.99	&	100	&	100	\\
8000	&	2	&	1	&	23.4	&	100	&	23.4	&	100	&	100	\\
8000	&	8	&	1	&	85.35	&	100	&	85.35	&	100	&	100	\\
8000	&	32	&	1	&	264.36	&	100	&	264.36	&	100	&	100	\\
8000	&	8	&	1	&	85.35	&	100	&	85.35	&	100	&	100	\\
8000	&	32	&	1	&	264.36	&	100	&	264.36	&	100	&	100	\\[1ex]
\hline                    % inserts single horizontal line 
\end{tabular}
\label{table:Power6_H1}  % is used to refer this table in the text 
\end{table}

\begin{table}[ht]
\caption{Performance of Heuristic~2 on the IBM Power6 machine.} % title of Table
\centering      % used for centering table 
\begin{tabular}{r r r r r r r r } % centered columns (4 columns) 
\hline\hline                        %inserts double horizontal lines 
N & ncore& Y &PS &$\frac{PS}{ES}\%$& PSPAYG & $\frac{PSPAYG}{ES}\%$&$\frac{PSPAYG}{PS}\%$\\ [0.5ex]
%heading 
\hline                    % inserts single horizontal line 
2000	&	8	&	1	&	55.97	&	100	&	55.97	&	100	&	100	\\
2000	&	32	&	1	&	85.14	&	100	&	85.14	&	100	&	100	\\
6000	&	8	&	1	&	81.67	&	100	&	81.67	&	100	&	100	\\
6000	&	32	&	1	&	255.83	&	100	&	255.83	&	100	&	100	\\
1000	&	1	&	1	&	9.23	&	100	&	9.23	&	100	&	100	\\
4000	&	1	&	1	&	11.44	&	100	&	11.44	&	100	&	100	\\
6000	&	1	&	1	&	11.72	&	100	&	11.72	&	100	&	100	\\
8000	&	1	&	1	&	12.05	&	100	&	12.05	&	100	&	100	\\
1000	&	2	&	1	&	14.85	&	100	&	14.85	&	100	&	100	\\
4000	&	2	&	1	&	21.83	&	100	&	21.83	&	100	&	100	\\
6000	&	2	&	1	&	22.99	&	100	&	22.99	&	100	&	100	\\
8000	&	2	&	1	&	23.4	&	100	&	23.4	&	100	&	100	\\
8000	&	8	&	1	&	85.35	&	100	&	85.35	&	100	&	100	\\
8000	&	32	&	1	&	264.36	&	100	&	264.36	&	100	&	100	\\
8000	&	8	&	1	&	85.35	&	100	&	85.35	&	100	&	100	\\
8000	&	32	&	1	&	264.36	&	100	&	264.36	&	100	&	100	\\[1ex]
\hline                    % inserts single horizontal line 
\end{tabular}
\label{table:Power6_H2}  % is used to refer this table in the text 
\end{table}
